# Supplementary material for: Embodied Visual Navigation with Automatic Curriculum Learning in Real Environments
Source: arXiv:2009.05429 source file (2021-01-06)
Supplement: Supplementary file 1 [file 6_supplemental.tex]

\appendix
\begin{comment}
%\section*{Supplemental material}
\section{Manifest}
The zip archive contains the following files:\\
\texttt{./appendix.pdf\\
./FinalVideos/AGV\_exp\_house\_orange\_ball\_480p.mp4\\
./FinalVideos/AGV\_exp\_house\_vase\_480p.mp4\\
./FinalVideos/AGV\_exp\_office\_480p.mp4\\
./FinalVideos/AGV\_exp\_house\_orange\_ball\_480p.mp4\\
./FinalVideos/Drone\_exp\_1\_480p.mp4\\
./FinalVideos/Drone\_exp\_2\_480p.mp4\\
./FinalVideos/Drone\_exp\_3\_480p.mp4
}
\end{comment}

\section{Video Results}
We provide video results from the collision-free AGV real-world tests (Tab. \ref{tab:real_results}) in the included \texttt{FinalVideos} directory. That directory also houses three videos of the UAV. All episodes of both the AGV and UAV are collision-free. We demonstrate semantic target-seeking behavior on the AGV and exploration behavior on the UAV. We show the agent observation (RGB image) and corresponding spatial and semantic features at each timestep, as well as the view from an external camera in some cases. The depth feature is postprocessed in the videos using histogram normalization to aid the viewer.

\texttt{AGV1.mp4} shows all AGV experiments in the Office 1 and Office 2 scenes. Other AGV videos showcase the ability to navigate to unseen objects (\texttt{AGV2.mp4}) and unseen classes (\texttt{AGV3.mp4}) in the House scene. The UAV videos show UAV exploring the Office 2 (\texttt{UAV1.mp4}, and \texttt{UAV3.mp4}) and Office 3 (\texttt{UAV2.mp4}) scenes. The UAVs flew until the battery was exhausted, hundreds of steps longer and much further than they saw in simulation.

\section{NavACL network details}
NavACL's $f_\pi$ is a feed-forward network with two hidden layers of size 64 with ReLU activation, learning rate 0.01, and binary cross-entropy loss. Learning rate, hidden layer size, and number of hidden layers were selected to minimize loss via grid search. The eight parameters used in geometric preprocessing of task $h=(s_0, s_g)$ come from easily accessible simulator metrics:
\begin{enumerate}
    \item Geodesic distance: The shortest-path distance from $s_0$ to $s_g$
    \item Path complexity: The ratio of euclidean distance to geodesic distance of $s_0,s_g$
    \item Sine of turn angle: The sine of the angle between the focal plane normal and the vector from the principal point to $s_g$ (\ie how much the agent must turn to see the goal)
    \item Cosine of turn angle: Similar to above, but using cosine
    \item Agent clearance: Distance from $s_0$ to the nearest obstacle
    \item Goal clearance: Distance from $s_g$ to the nearest obstacle
    \item Agent island: Radius of the traversable area at $s_0$
    \item Goal island: Radius of the traversable area at $s_g$
\end{enumerate}

\section{NavACL and GoalGAN comparison}
We compare the effectiveness of NavACL-GOID with GoalGAN. Both methods are designed to output GOID tasks. GoalGAN uses the same implementation and parameters as the \emph{MazeAnt} 3D navigation example in \citet{florensa2018automatic}, with a batch size of 100 episodes. $s_0, s_g$ coming from GoalGAN are not guaranteed to be valid points in the scene, so they are ``snapped'' to the nearest traversable point in the navmesh, up to a distance of $5.5$m. $s_0,s_g$ are considered valid if both $s_0$ and $s_g$ are traversable and there exists a continuous traversable path connecting them. If GoalGAN generates an invalid sample, we redraw samples until we obtain a valid sample. We give up drawing samples after one hundred invalid tasks per episode, providing a valid random task instead. Tasks within $0.5$m of each other are binned to estimate success probability labels for GoalGAN training. 

NavACL-GOID targets tasks with estimated success probability $0.4 \leq f_\pi(h) \leq 0.6$. We evaulate GoalGAN using both $0.4 \leq f_{GoalGAN}(h) \leq 0.6$ (our default NavACL-GOID target) and $0.1 \leq f_{GoalGAN}(h) \leq 0.9$ (\citet{florensa2018automatic} recommended target), where  $f_{GoalGAN}(h)$ is the GoalGAN estimated success probability of task $h$. Due to time constraints, we were only able to run a single trial for each GoalGAN setup. We provide results in Fig. \ref{fig:goalgan}.

Roughly halfway through testing we found $0.1 \leq f_{GoalGAN}(h) \leq 0.9$ collapsed -- it was not able to provide viable $s_0, s_g$, and so the agent received almost entirely random tasks from then on. By that point, ACL had served its purpose and the agent was able to learn from random tasks (the logic behind NavACL-adaptive). We find both NavACL-GOID and GoalGAN help overcome sparse rewards to produce viable agents, with GoalGAN taking more wall-clock time for training and inference than NavACL (Fig. \ref{tab:perf}).

\begin{figure}
    \centering
    \begin{subfigure}{0.5\linewidth}
    \includegraphics[width=\linewidth]{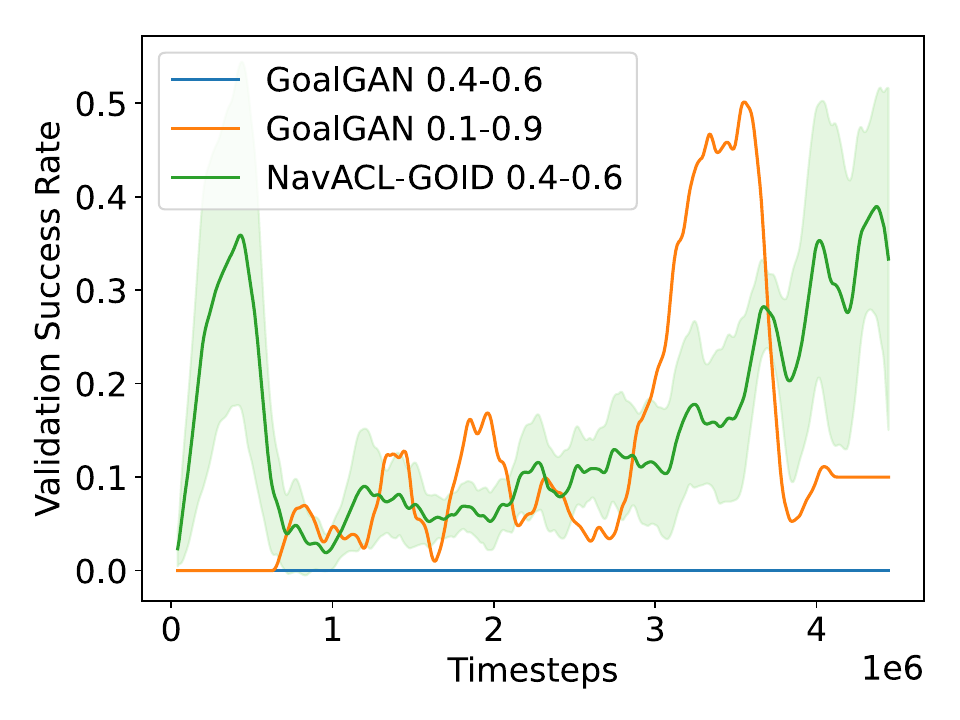}
    \caption{NavACL-GOID and GoalGAN applied to visual navigation. The number ranges denote the task success probabilities labeled as intermediate difficulty.}
    \label{fig:goalgan}
    \end{subfigure}
    \begin{subtable}{0.45\linewidth}
    \centering
    \begin{tabular}{ccc}
    & Train (s) & Inference (s)\\
    \hline
    NavACL & 0.002 & 0.017\\
    GoalGAN & 0.019 & 0.035\\ 
    \end{tabular}
    \caption{ACL per-episode mean wall-clock times}
    \label{tab:perf}
\end{subtable}
\caption{Comparison of GoalGAN and NavACL-GOID}
\end{figure}

\section{Model network details}
Our feature compressor network is a three-layer CNN which takes as input $1 \times (8n+1) \times 16 \times 16$ matrices where $n$ is the number of spatial features, and compresses them using convolutional layers with ReLU activation (Tab. \ref{tab:feat_comp}). The compressed representation feeds into a 256-node LSTM. The LSTM hidden state is reset between episodes. The LSTM feeds into a fully connected output layer that produces the agent action and the value estimate of the current state. The PPO parameters we used to optimize our policies are available in Tab. \ref{tab:param}.

\begin{table}
    \caption{Policy details}
    \begin{subtable}[t]{0.5\linewidth}
        \centering
        \caption{Feature compressor network architecture}
        \begin{tabular}{cccc}
            Layer & Num. Filters & Kernel Size & Stride\\
            \hline
            1 & 32 & 4 & 2\\
            2 & 64 & 4 & 2\\
            3 & 128 & 2 & 1
        \end{tabular}
        \label{tab:feat_comp}
    \end{subtable}
    \begin{subtable}[t]{0.5\linewidth}
    \centering
    \caption{PPO hyperparameters used to train our policy}
    \label{tab:param}
    \vspace{1em}
    \begin{tabular}{lr}
        number of minibatches & 1\\
        learning rate & 0.005\\
        clipping range $(\epsilon)$ & 0.10 \\
        discount factor $(\gamma)$ & 0.99 \\
        value fuction coefficient $(c_1)$ & 0.5\\
        entropy coefficient $(\beta \text{ or } c_2)$ & 0.01 \\
        timesteps per policy update & 4000 \\
        rollout workers & 12\\
        inner-loop epochs & 4\\
        GAE $\lambda$ & 0.95\\
    \end{tabular}
\end{subtable}
\end{table}

\begin{comment}
\begin{table}
    \centering
    \caption{PPO hyperparameters used to train our policy}
    \vspace{1em}
    \begin{tabular}{lr}
        number of minibatches & 1\\
        learning rate & 0.005\\
        clipping range $(\epsilon)$ & 0.10 \\
        discount factor $(\gamma)$ & 0.99 \\
        value fuction coefficient $(c_1)$ & 0.5\\
        entropy coefficient $(\beta \text{ or } c_2)$ & 0.01 \\
        timesteps per policy update & 4000 \\
        rollout workers & 12\\
        inner-loop epochs & 4\\
        GAE $\lambda$ & 0.95\\
    \end{tabular}
    \label{tab:param}
\end{table}
\end{comment}
